# Supplementary material for: Berry Population Analysis: Atomic Charges from the Berry Curvature in a Magnetic Field
Source: arXiv:2211.07240 source file (2022-11-14)
Supplement: Supplementary file 1 [file si.pdf]

# Berry Population Analysis:
# Atomic Charges from the Berry Curvature in a Magnetic Field
# – Supporting Information

Laurens D. M. Peters,[1, a)] Tanner P. Culpitt,[1] Erik I. Tellgren,[1] and Trygve Helgaker[1]

*Hylleraas Centre for Quantum Molecular Sciences, Department of Chemistry, University of Oslo, P.O. Box 1033 Blindern, N-0315 Oslo, Norway*

(Dated: 14 November 2022)

[a)] Electronic mail: laurens.peters@kjemi.uio.no

## CONTENTS


I. Convergence of Numerical Spherical Integration 3

II. Rotationally Averaged Atomic Charges 4

References 8

## I. CONVERGENCE OF NUMERICAL SPHERICAL INTEGRATION

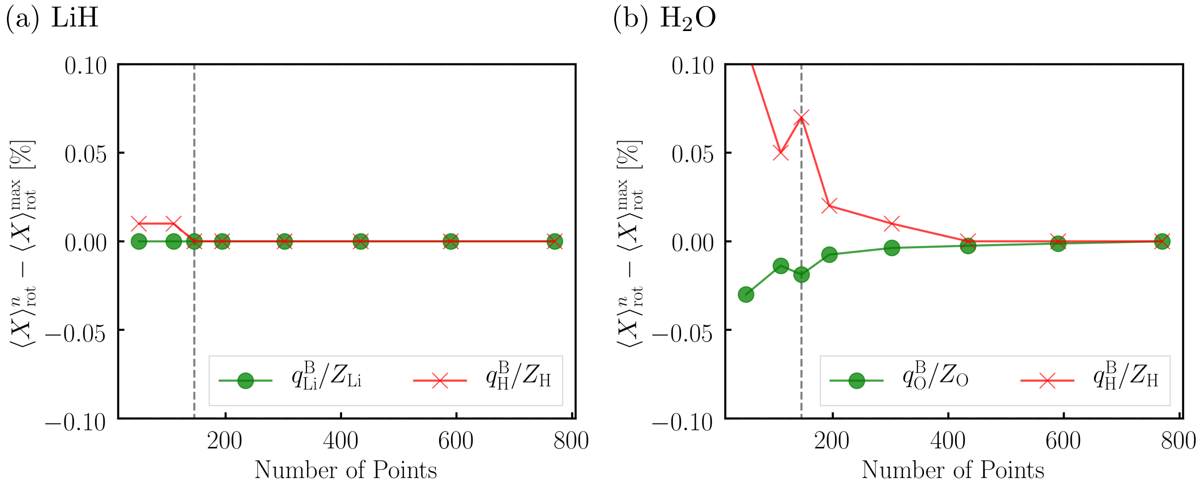


FIG. 1: Convergence of rotationally averaged charges of LiH (a) and $H_2O$ (b) with the number of grid points $n$ for the numerical spherical integration. All calculations were performed at the HF/cc-pVDZ/$\mathbf{B} = 0.001\ B_0$ level of theory. Grid points and weights were taken from the QUADPY[1] program package. Our desired accuracy and choice for this work are indicated by horizontal and vertical dashed lines, respectively. The final point was set to zero.

## II. ROTATIONALLY AVERAGED ATOMIC CHARGES

TABLE I: Rotationally averaged atomic charges ($q_I$, in $e$) of different molecules obtained from Berry (B), atomic-polar-tensor (D), and Mulliken (M) population analyses. All values were obtained at the HF/cc-pVDZ/$\mathbf{B} = 0.001\ B_0$ level of theory using 146 grid points/weights taken from the QUADPY[1] program package.

| Molecule | $I$ | $\langle q_I^{\mathrm{B}} \rangle$ | $\langle q_I^{\mathrm{D}} \rangle$ | $\langle q_I^{\mathrm{M}} \rangle$ |
|---|---|---|---|---|
| LiF | F | -0.8109 | -0.8270 | -0.6227 |
| | Li | 0.8110 | 0.8270 | 0.6227 |
| $BeF_2$ | Be | 1.4251 | 1.3766 | 0.8211 |
| | F | -0.7124 | -0.6883 | -0.4105 |
| | F | -0.7124 | -0.6883 | -0.4105 |
| $BF_3$ | B | 1.9261 | 1.8620 | 0.6142 |
| | F | -0.6121 | -0.6207 | -0.2047 |
| | F | -0.6568 | -0.6207 | -0.2047 |
| | F | -0.6568 | -0.6207 | -0.2047 |
| $CF_4$ | F | -0.5641 | -0.5837 | -0.2059 |
| | C | 2.2568 | 2.3346 | 0.8235 |
| | F | -0.5257 | -0.5837 | -0.2059 |
| | F | -0.5832 | -0.5837 | -0.2059 |
| | F | -0.5832 | -0.5837 | -0.2059 |
| $NH_3$ | N | 1.1867 | 1.3094 | 0.5756 |
| | F | -0.3542 | -0.4365 | -0.1919 |
| | F | -0.4160 | -0.4365 | -0.1919 |
| | F | -0.4160 | -0.4365 | -0.1919 |
| $OF_2$ | O | 0.3526 | 0.4545 | 0.2158 |
| | F | -0.1761 | -0.2273 | -0.1079 |
| | F | -0.1761 | -0.2273 | -0.1079 |
| $F_2$ | F | 0.0001 | -0.0000 | 0.0000 |
| | F | 0.0001 | -0.0000 | 0.0000 |
| $LiCH_3$ | C | -0.3462 | -0.3998 | -0.3230 |
| | Li | 0.6761 | 0.6716 | 0.3052 |
| | H | -0.1047 | -0.0906 | 0.0059 |
| | H | -0.1047 | -0.0906 | 0.0059 |
| | H | -0.1204 | -0.0906 | 0.0059 |

TABLE II: Rotationally averaged atomic charges ($q_I$, in $e$) of different molecules obtained from Berry (B), atomic-polar-tensor (D), and Mulliken (M) population analyses. All values were obtained at the HF/cc-pVDZ/$\mathbf{B} = 0.001\ B_0$ level of theory using 146 grid points/weights taken from the QUADPY[1] program package.

| Molecule | $I$ | $\langle q_I^{\mathrm{B}} \rangle$ | $\langle q_I^{\mathrm{D}} \rangle$ | $\langle q_I^{\mathrm{M}} \rangle$ |
|---|---|---|---|---|
| $BeHCH_3$ | C | -0.3117 | -0.3780 | -0.1443 |
| | Be | 0.7245 | 0.7902 | 0.1882 |
| | H | -0.0306 | -0.0067 | 0.0286 |
| | H | -0.0101 | -0.0067 | 0.0286 |
| | H | -0.0136 | -0.0067 | 0.0286 |
| | H | -0.3585 | -0.3920 | -0.1298 |
| $BH_2CH_3$ | C | -0.1755 | -0.2108 | -0.1571 |
| | B | 0.5735 | 0.6911 | 0.1839 |
| | H | -0.0091 | 0.0027 | 0.0414 |
| | H | -0.0115 | -0.0226 | 0.0325 |
| | H | -0.0091 | 0.0027 | 0.0414 |
| | H | -0.1851 | -0.2362 | -0.0707 |
| | H | -0.1832 | -0.2269 | -0.0713 |
| $CH_3CH_3$ | C | 0.1224 | 0.1417 | -0.0886 |
| | C | 0.1224 | 0.1417 | -0.0886 |
| | H | -0.0487 | -0.0472 | 0.0295 |
| | H | -0.0251 | -0.0472 | 0.0295 |
| | H | -0.0487 | -0.0472 | 0.0295 |
| | H | -0.0251 | -0.0472 | 0.0295 |
| | H | -0.0487 | -0.0472 | 0.0295 |
| | H | -0.0487 | -0.0472 | 0.0295 |
| $CH_3NH_2$ | C | 0.3043 | 0.4270 | 0.0471 |
| | N | -0.3550 | -0.4728 | -0.2922 |
| | H | -0.0207 | -0.0487 | 0.0325 |
| | H | -0.0207 | -0.0487 | 0.0325 |
| | H | -0.0970 | -0.1114 | 0.0071 |
| | H | 0.0946 | 0.1273 | 0.0865 |
| | H | 0.0946 | 0.1273 | 0.0865 |
| $CH_3OH$ | C | 0.4516 | 0.6094 | 0.1467 |
| | O | -0.5574 | -0.6767 | -0.3594 |
| | H | -0.0446 | -0.0876 | 0.0118 |
| | H | -0.0202 | -0.0366 | 0.0386 |
| | H | -0.0446 | -0.0876 | 0.0118 |
| | H | 0.2155 | 0.2791 | 0.1504 |
| $CH_3F$ | C | 0.6176 | 0.7030 | 0.2478 |
| | F | -0.5629 | -0.5692 | -0.3358 |
| | H | -0.0120 | -0.0446 | 0.0293 |
| | H | -0.0304 | -0.0446 | 0.0293 |
| | H | -0.0120 | -0.0446 | 0.0293 |

TABLE III: Rotationally averaged atomic charges ($q_I$, in $e$) of different molecules obtained from Berry (B), atomic-polar-tensor (D), and Mulliken (M) population analyses. All values were obtained at the HF/cc-pVDZ/$\mathbf{B} = 0.001\ B_0$ level of theory using 146 grid points/weights taken from the QUADPY[1] program package.

| Molecule | $I$ | $\langle q_I^{\mathrm{B}} \rangle$ | $\langle q_I^{\mathrm{D}} \rangle$ | $\langle q_I^{\mathrm{M}} \rangle$ |
|---|---|---|---|---|
| LiH | Li | 0.6063 | 0.6604 | 0.1254 |
| | H | -0.6063 | -0.6604 | -0.1254 |
| BeH2 | Be | 0.6795 | 0.7446 | 0.2260 |
| | H | -0.3399 | -0.3723 | -0.1130 |
| | H | -0.3399 | -0.3723 | -0.1130 |
| $BH_3$ | B | 0.5673 | 0.6041 | 0.1575 |
| | H | -0.1816 | -0.2014 | -0.0525 |
| | H | -0.1928 | -0.2014 | -0.0525 |
| | H | -0.1928 | -0.2014 | -0.0525 |
| $CH_4$ | H | -0.0138 | -0.0156 | 0.0369 |
| | C | 0.0551 | 0.0624 | -0.1477 |
| | H | -0.0271 | -0.0156 | 0.0369 |
| | H | -0.0071 | -0.0156 | 0.0369 |
| | H | -0.0071 | -0.0156 | 0.0369 |
| $NH_3$ | N | -0.2791 | -0.4207 | -0.2561 |
| | H | 0.0783 | 0.1402 | 0.0854 |
| | H | 0.1005 | 0.1402 | 0.0854 |
| | H | 0.1005 | 0.1402 | 0.0854 |
| $H_2O$ | O | -0.4219 | -0.5605 | -0.2897 |
| | H | 0.2110 | 0.2802 | 0.1449 |
| | H | 0.2110 | 0.2802 | 0.1449 |
| HF | F | -0.4079 | -0.4332 | -0.2230 |
| | H | 0.4081 | 0.4332 | 0.2230 |

TABLE IV: Rotationally averaged atomic charges ($q_I$, in $e$) of different molecules obtained from Berry (B), atomic-polar-tensor (D), and Mulliken (M) population analyses. All values were obtained at the HF/cc-pVDZ/$\mathbf{B} = 0.001\ B_0$ level of theory using 146 grid points/weights taken from the QUADPY[1] program package.

| Molecule | $I$ | $\langle q_I^{\mathrm{B}} \rangle$ | $\langle q_I^{\mathrm{D}} \rangle$ | $\langle q_I^{\mathrm{M}} \rangle$ |
|---|---|---|---|---|
| $Li_2$ | Li | 0.0013 | 0.0000 | 0.0000 |
| | Li | 0.0013 | 0.0000 | 0.0000 |
| LiBeH | Be | -0.0809 | -0.0424 | 0.1422 |
| | Li | 0.3303 | 0.3358 | 0.0138 |
| | H | -0.2495 | -0.2933 | -0.1560 |
| $LiBH_2$ | B | -0.2196 | -0.1341 | 0.0635 |
| | Li | 0.5141 | 0.5244 | 0.1174 |
| | H | -0.1474 | -0.1951 | -0.0904 |
| | H | -0.1474 | -0.1951 | -0.0904 |
| $LiNH_2$ | N | -0.6570 | -0.8624 | -0.5295 |
| | Li | 0.6992 | 0.7170 | 0.4103 |
| | H | -0.0210 | 0.0727 | 0.0596 |
| | H | -0.0210 | 0.0727 | 0.0596 |
| LiOH | O | -0.8622 | -1.0174 | -0.6403 |
| | Li | 0.7278 | 0.7786 | 0.5158 |
| | H | 0.1345 | 0.2388 | 0.1246 |

**REFERENCES**

[1] "quadpy 0.16.14, Numerical integration, quadrature for various domains. By N. Schlömer See https://pypi.org/project/quadpy/ for more information.".
